# Supplementary material for: AgentDroid: A Multi-Agent Framework for Detecting Fraudulent Android Applications
Source: arXiv:2503.12163 source file (2025-10-08)
Supplement: Supplementary file 1 [file Appendix.tex]

\newpage

\section*{Appendix}
\appendix

\section{Prompts}

% \begin{figure*}[]
% \centering
% \includegraphics[width=\textwidth]{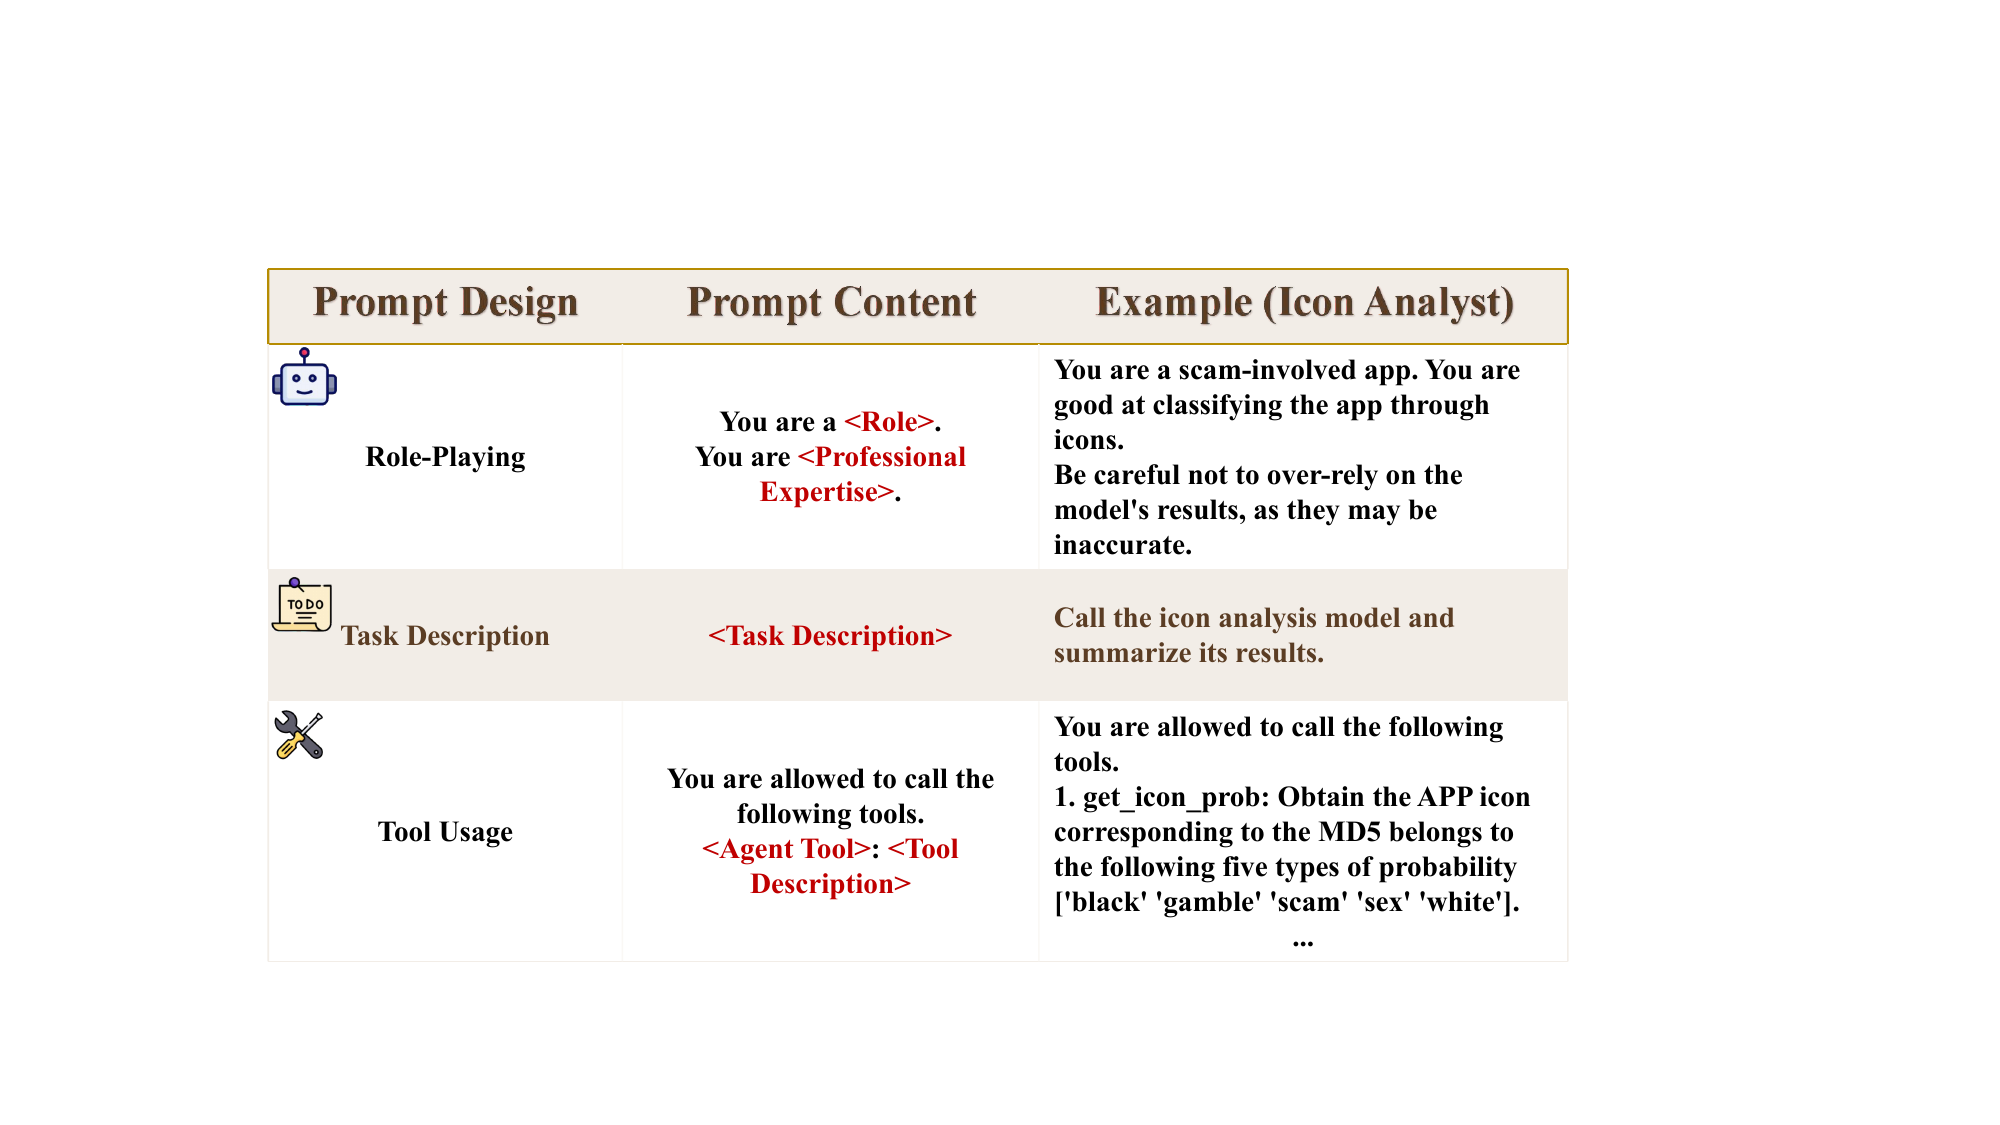} % 使用双栏宽度
% \caption{System prompts of AgentDroid (All the Prompts and Agent Interaction Examples are available in the \href{https://anonymous.4open.science/r/AgentDroid/}{\textit{Repository}})\hy{can move this to the previous page}}
% \label{fig:prompt}
% \end{figure*}

AgentDroid consists of eight agents (Task Master, Package Tracer, Icon Analyst, Permission Analyst, Content Analyst, Certificate Checker, Link Analyst, and Decision Maker), whose prompts are illustrated in Figure \ref{fig:prompt}.

% \clearpage
% \begin{figure*}[h]
% \centering
% \includegraphics[width=\textwidth]{prompt.pdf}
% \caption{System prompts of AgentDroid (All the Prompts and Agent Interaction Examples are available in the \href{https://anonymous.4open.science/r/AgentDroid/}{\textit{Repository}})}
% \label{fig:prompt}
% \end{figure*}

% \noindent
% \makebox[\textwidth][c]{%
%     \includegraphics[width=\textwidth]{prompt.pdf}
% }
% \captionof{figure}{System prompts of AgentDroid (All the Prompts and Agent Interaction Examples are available in the \href{https://anonymous.4open.science/r/AgentDroid/}{\textit{Repository}})}
% \label{fig:prompt}

\noindent
\begin{minipage}{\textwidth} % 设置为双栏宽度
    \makebox[\textwidth][c]{%
        \includegraphics[width=\textwidth]{prompt.pdf}
    }
    \captionof{figure}{System prompts of AgentDroid (All the Prompts and Agent Interaction Examples are available in our project \href{https://anonymous.4open.science/r/AgentDroid/}{\textit{Repository}})}
    \label{fig:prompt}
\end{minipage}
